# Supplementary material for: CMA-ES with Adaptive Reevaluation for Multiplicative Noise
Source: arXiv:2405.11471 source file (2024-05-19)
Supplement: Supplementary file 1 [file supplement.pdf]

# CMA-ES with Adaptive Reevaluation for Multiplicative Noise: Supplementary Material

Kento Uchida  
uchida-kento-fz@ynu.ac.jp  
Yokohama National University  
Yokohama, Kanagawa, Japan

Kenta Nishihara  
nishihara-kenta@ynu.jp  
Yokohama National University  
Yokohama, Kanagawa, Japan

Shinichi Shirakawa  
shirakawa-shinichi-bg@ynu.ac.jp  
Yokohama National University  
Yokohama, Kanagawa, Japan

## ACM Reference Format:

Kento Uchida, Kenta Nishihara, and Shinichi Shirakawa. 2018. CMA-ES with Adaptive Reevaluation for Multiplicative Noise: Supplementary Material. In *Woodstock '18: ACM Symposium on Neural Gaze Detection, June 03–05, 2018, Woodstock, NY*. ACM, New York, NY, USA, 2 pages. <https://doi.org/10.1145/1122445.1122456>

## A PROOF OF LEMMAS

### A.1 Proof of Lemma 3.1

PROOF. Let us consider the objective function in the form  $f(\mathbf{x}, z) = z f_{\mathbf{x}}(\mathbf{x}) + b$  with a constant value  $b \in \mathbb{R}$ . We consider the case that the noise  $z$  takes 1 or  $-1$  only, i.e.  $z \in \{-1, 1\}$ , and given independently from  $\mathbf{x}$ . We will construct a function  $f_{\mathbf{x}}$  satisfying

$$\mathbf{x}^* \notin \arg \max_{\mathbf{x} \in \mathcal{X}} \mathbb{E}_{z|\mathbf{x}}[v(\mathbf{x}, z; \theta)] . \quad (1)$$

with convex and concave selection scheme  $w$  separately.

*Convex case:* Consider the objective function is given by

$$f_{\mathbf{x}}(\mathbf{x}) = \begin{cases} 0 & \text{if } \mathbf{x} = \mathbf{x}^* \\ 1 & \text{otherwise} \end{cases} . \quad (2)$$

Considering  $\Pr_{\mathbf{x}' \sim p_{\theta}}(\mathbf{x}' \neq \mathbf{x}^*) = 1$ , the quantiles  $q_v^<$  and  $q_v^{\leq}$  are given by

$$q_v^<(\mathbf{x}, z) = \begin{cases} p_z^- & \text{if } \mathbf{x} = \mathbf{x}^* \\ 0 & \text{if } \mathbf{x} \neq \mathbf{x}^* \text{ and } z = -1 \\ p_z^- & \text{if } \mathbf{x} \neq \mathbf{x}^* \text{ and } z = 1 \end{cases} \quad (3)$$

$$q_v^{\leq}(\mathbf{x}, z) = \begin{cases} p_z^- & \text{if } \mathbf{x} = \mathbf{x}^* \\ p_z^- & \text{if } \mathbf{x} \neq \mathbf{x}^* \text{ and } z = -1 \\ 1 & \text{if } \mathbf{x} \neq \mathbf{x}^* \text{ and } z = 1 \end{cases} . \quad (4)$$

Permission to make digital or hard copies of all or part of this work for personal or classroom use is granted without fee provided that copies are not made or distributed for profit or commercial advantage and that copies bear this notice and the full citation on the first page. Copyrights for components of this work owned by others than ACM must be honored. Abstracting with credit is permitted. To copy otherwise, or republish, to post on servers or to redistribute to lists, requires prior specific permission and/or a fee. Request permissions from [permissions@acm.org](mailto:permissions@acm.org).

Woodstock '18, June 03–05, 2018, Woodstock, NY

© 2018 Association for Computing Machinery.

ACM ISBN 978-1-4503-XXXX-X/18/06...\$15.00

<https://doi.org/10.1145/1122445.1122456>

where we denote  $p_z^- = \Pr_{z' \sim p_n}(z' = -1)$  for short. The utility value is determined for  $\mathbf{x}^*$  and  $\mathbf{x}' \neq \mathbf{x}^*$  as

$$v(\mathbf{x}^*, z; \theta) = w(p_z^-) \quad (5)$$

$$v(\mathbf{x}', -1; \theta) = \frac{1}{p_z^-} \int_0^{p_z^-} w(q) dq \quad (6)$$

$$v(\mathbf{x}', 1; \theta) = \frac{1}{1 - p_z^-} \int_{p_z^-}^1 w(q) dq \quad (7)$$

The expected utility is given by

$$\mathbb{E}_{z|\mathbf{x}}[v(\mathbf{x}, z; \theta) | \mathbf{x} = \mathbf{x}^*] = w(\Pr(z = -1)) \quad (8)$$

$$\begin{aligned} \mathbb{E}_{z|\mathbf{x}}[v(\mathbf{x}, z; \theta) | \mathbf{x} \neq \mathbf{x}^*] \\ = \int_0^{p_z^-} w(q) dq + \int_{p_z^-}^1 w(q) dq = \int_0^1 w(q) dq . \end{aligned} \quad (9)$$

Since  $w$  is strictly convex, Jensen's inequality shows that there exists  $\epsilon > 0$  that holds

$$\int_0^1 w(q) dq = w\left(\frac{1}{2}\right) + \epsilon . \quad (10)$$

Moreover, we can consider arbitrary small  $\delta \in (0, 1/2)$  which satisfies  $p_z^- = \Pr(z = -1) = 1/2 - \delta$ . We have

$$\begin{aligned} \mathbb{E}_{z|\mathbf{x}}[v(\mathbf{x}, z; \theta) | \mathbf{x} \neq \mathbf{x}^*] - \mathbb{E}_{z|\mathbf{x}}[v(\mathbf{x}, z; \theta) | \mathbf{x} = \mathbf{x}^*] \\ = \int_0^1 w(q) dq - w(p_z^-) \end{aligned} \quad (11)$$

$$= \epsilon - \left( w\left(\frac{1}{2} - \delta\right) - w\left(\frac{1}{2}\right) \right) \quad (12)$$

Since  $w$  is convex function on the open interval  $(0, 1)$ , it is continuous on  $(0, 1)$ . Therefore, for any  $\epsilon$ , there exists  $\delta > 0$  which holds

$$\mathbb{E}_{z|\mathbf{x}}[v(\mathbf{x}, z; \theta) | \mathbf{x} \neq \mathbf{x}^*] > \mathbb{E}_{z|\mathbf{x}}[v(\mathbf{x}, z; \theta) | \mathbf{x} = \mathbf{x}^*] . \quad (13)$$

*Concave case:* Consider the objective function is given by

$$f_{\mathbf{x}}(\mathbf{x}) = \begin{cases} -1 & \text{if } \mathbf{x} = \mathbf{x}^* \\ 0 & \text{otherwise} \end{cases} . \quad (14)$$

In this case, the quantiles  $q^<$  and  $q^{\leq}$  are give by

$$q^<(\mathbf{x}, z) = \begin{cases} 0 & \text{if } \mathbf{x} = \mathbf{x}^* \text{ and } z = 1 \\ 1 & \text{if } \mathbf{x} = \mathbf{x}^* \text{ and } z = -1 \\ 1 & \text{otherwise} \end{cases} \quad (15)$$

$$q^{\leq}(\mathbf{x}, z) = \begin{cases} 0 & \text{if } \mathbf{x} = \mathbf{x}^* \text{ and } z = 1 \\ 1 & \text{if } \mathbf{x} = \mathbf{x}^* \text{ and } z = -1 \\ 0 & \text{otherwise} \end{cases} . \quad (16)$$

Then, the expected utility is given by

$$\mathbb{E}_{\mathbf{z}|\mathbf{x}}[v(\mathbf{x}, \mathbf{z}; \theta) \mid \mathbf{x} = \mathbf{x}^*] = \Pr(z = 1)w(0) + \Pr(z = -1)w(1) \quad (17)$$

$$\mathbb{E}_{\mathbf{z}|\mathbf{x}}[v(\mathbf{x}, \mathbf{z}; \theta) \mid \mathbf{x} \neq \mathbf{x}^*] = \int_0^1 w(q) dq \quad (18)$$

For strictly concave function, we have

$$\int_0^1 w(q) dq > \int_0^1 ((1-q)w(0) + qw(1)) dq \quad (19)$$

$$= \frac{3}{4}w(0) + \frac{1}{4}w(1) \quad (20)$$

Therefore, setting  $\Pr(z = 1) = 3/4$  satisfies

$$\mathbb{E}_{\mathbf{z}|\mathbf{x}}[v(\mathbf{x}, \mathbf{z}; \theta) \mid \mathbf{x} \neq \mathbf{x}^*] > \mathbb{E}_{\mathbf{z}|\mathbf{x}}[v(\mathbf{x}, \mathbf{z}; \theta) \mid \mathbf{x} = \mathbf{x}^*] \quad (21)$$

This is end of the proof.  $\square$

## A.2 Proof of Lemma 3.2

PROOF. Because the probability of the event  $f(\mathbf{x}, \mathbf{z}) = f(\mathbf{x}', \mathbf{z}')$  is zero for any  $\mathbf{x}$  and  $\mathbf{x}'$  under additive Gaussian noise, we have

$$\mathbb{E}_{\mathbf{z}|\mathbf{x}}[v(\mathbf{x}, \mathbf{z}; \theta)] = \mathbb{E}_{\mathbf{z}|\mathbf{x}}[w(q_v^<(\mathbf{x}, \mathbf{z}; \theta))] \quad (22)$$

$$= \mathbb{E}_{\mathbf{z}|\mathbf{x}} \left[ w \left( \Pr_{\mathbf{x}', \mathbf{z}' \sim \hat{P}_\theta} (f(\mathbf{x}', \mathbf{z}') < f(\mathbf{x}, \mathbf{z})) \right) \right] \quad (23)$$

Fixing the noise  $\mathbf{z}$ , an optimal solution  $\mathbf{x}^*$  satisfies  $f(\mathbf{x}^*, \mathbf{z}) \leq f(\mathbf{x}, \mathbf{z})$  for any  $\mathbf{x}$ , and we have

$$\Pr_{\mathbf{x}', \mathbf{z}' \sim \hat{P}_\theta} (f(\mathbf{x}', \mathbf{z}') < f(\mathbf{x}^*, \mathbf{z})) \leq \Pr_{\mathbf{x}', \mathbf{z}' \sim \hat{P}_\theta} (f(\mathbf{x}', \mathbf{z}') < f(\mathbf{x}, \mathbf{z}))$$

Finally, because the selection scheme  $w$  is non-increasing function, it holds for any  $\mathbf{x}$  as

$$\mathbb{E}_{\mathbf{z}|\mathbf{x}}[v(\mathbf{x}^*, \mathbf{z}; \theta)] \geq \mathbb{E}_{\mathbf{z}|\mathbf{x}}[v(\mathbf{x}, \mathbf{z}; \theta)] \quad (24)$$

This is end of the proof.  $\square$

## A.3 Proof of Lemma 3.3

PROOF. Because the optimal solution  $\mathbf{x}^*$  is unique, we have  $q_u^<(\mathbf{x}^*; \theta) = q_u^<(\mathbf{x}^*; \theta) = 0$  for any  $\theta \in \Theta$ . Then, reminding the utility function  $u(\cdot; \theta)$  is non-increasing w.r.t.  $q_u^<(\cdot; \theta)$ , the proof is finished.  $\square$
